# Supplementary material for: TACCO: Task-guided Co-clustering of Clinical Concepts and Patient Visits for Disease Subtyping based on EHR Data
Source: arXiv:2406.10061 source file (2024-06-14)
Supplement: Supplementary file 1 [file appendix.tex]

% appendix.tex
\newpage
\appendix
\section{Additional Results}

\subsection{How Do Different Deep Clustering Methods Perform?}
\zy{need a table here}
\subsection{Hyperparameter Study on CRADLE}
\zy{need a figure here}

\subsection{Efficiency Study}
\zy{need a figure here}

\section{Deployment Status}
